# Supplementary material for: Bringing Clustering to MLL: Weakly-Supervised Clustering for Partial Multi-Label Learning
Source: arXiv:2604.09359 source file (2026-04-10)
Supplement: Supplementary file 1 [file X_suppl.tex]

\clearpage
\setcounter{page}{1}

\appendix
 % Switch to alphabetic numbering

\section{Motivation}

In general-domain datasets, captions involve millions of unique objects, scenes, and entities interacting in a multitude of combinations. Due to the diverse nature of general-domain data, contrastive learning is highly effective, as diversity is guaranteed even with random sampling of data into a batch. However, in medical settings, there are far fewer entities, and their relationships are limited, which does not align well with the objectives of contrastive learning.

\subsection{Imbalance}
Clinical data is often highly skewed, containing many duplicate templated reports, as shown in \cref{tab:skew}. Even when reports differ slightly in wording, semantically identical information still limits the effectiveness of standard contrastive learning. This has led many medical researchers and companies to discard duplicates and train models in a more balanced setting. However, fully normal chest X-rays (CXRs) contain crucial information for triage in clinical practice, as identifying normal cases can significantly reduce radiologists' workload. Our goal, therefore, is to develop a method that leverages all data—including duplicates—without discarding valuable information.

Furthermore, many reports are semantically similar even if the textual expressions differ. This occurs because there is an imbalance in the entities themselves; similar symptoms are commonly found across medical reports. This can cause semantic overlaps within a batch, where larger batch sizes might introduce more complexity in a contrastive learning context. As illustrated in \cref{fig:all_entity}, when trained with clinical data, one must consider this imbalance of clinical findings within the dataset. Using a general hospital dataset—which has more long-tailed characteristics compared to public data—could introduce noise into the training process due to this imbalance.

\begin{table}[h!]
\centering
 % Adjust row spacing for readability
\begin{tabular}{|p{0.8\columnwidth}|r|}
\hline
\multicolumn{2}{|c|}{\textbf{Impression}} \\
\hline
No acute cardiopulmonary process. & 37,962 \\
\hline
No acute cardiopulmonary abnormality. & 10,806 \\
\hline
No acute intrathoracic process. & 10,744 \\
\hline
\multicolumn{2}{|c|}{\textbf{Findings}} \\
\hline
Heart size is normal. The mediastinal and hilar contours are normal. The pulmonary vasculature is normal. Lungs are clear. No pleural effusion or pneumothorax is seen. There are no acute osseous abnormalities. & 2,209 \\
\hline
PA and lateral views of the chest provided. There is no focal consolidation, effusion, or pneumothorax. The cardiomediastinal silhouette is normal. Imaged osseous structures are intact. No free air below the right hemidiaphragm is seen. & 1,763 \\
\hline
The lungs are clear without focal consolidation. No pleural effusion or pneumothorax is seen. The cardiac and mediastinal silhouettes are unremarkable. & 1,635 \\
\hline
\end{tabular}
\caption{Most frequent reports from MIMIC impressions and findings. Note that the counts differ from \cref{tab:report_counts} since the reports used in training prioritize findings over impressions.}
\label{tab:skew}
\end{table}

\begin{figure}[t]
    \centering
    \includegraphics[width=1\linewidth]{graphics/counts_entity.png}
    \caption{Counts of clinical entities in the whole MIMIC training set and a private dataset collected from a tertiary hospital. The private dataset comprises around 1.3 million records collected over 20 years, each from unique patients.}
    \label{fig:all_entity}
\end{figure}

\subsection{Similarity}
\label{sec:motive}
Standard contrastive learning frameworks typically pull positive pairs together and push negative pairs apart. From a clinical perspective, it would be beneficial if similarity could be weighted according to clinical context. For instance, a report noting “Right large pleural effusion. No pneumothorax.” should be considered closer to “Right small pleural effusion.” than to “No pleural effusion. Cardiomegaly exists,” reflecting the clinical relevance of both findings. This is why we incorporate soft labels using similarity measures rather than a uniform distribution of soft labels, which has already been shown to be beneficial in~\cite{softclip}. Notably, using this characteristic, we can also handle duplicates or overlaps of clinical semantics since this method shares labels with similar or identical data within the batch.

We explore three types of similarity—textual, clinical, and graph-based—to achieve this nuanced approach. Similarity measures play a crucial role in contrastive learning, particularly in the medical domain. The SOFTCLIP~\cite{softclip} method, which also uses soft labels, relies primarily on textual similarity and is not well-suited for medical data where textual and clinical meanings often diverge. As shown in \cref{fig:similarity}, textual similarity alone does not align well with clinical importance. For example, for the report “Mild cardiomegaly. The lungs are clear,” the textual similarity score is higher with “The cardiomediastinal silhouette is normal. The lungs are clear.” than with “The cardiac silhouette is moderately enlarged. No pleural effusion.” Although the latter is closer in clinical meaning, textual similarity alone fails to capture this. Therefore, using solely textual similarity as soft labels can inadvertently bring unrelated reports closer rather than pushing them apart. This effect is demonstrated in \cref{ex:main} where SOFTCLIP performs worse than the baseline model.

While clinical similarity captures context better than text alone, it does not account for critical details like severity or location, such as “severe” or “mild.” To address this, we introduce graph similarity, which can capture these nuanced attributes and improve alignment.

\begin{figure}[t]
    \centering
    \includegraphics[width=1\linewidth]{graphics/entities_report.PNG}
    \caption{Counts of clinical entities in reports for the MIMIC training set.}
    \label{fig:entity_value_counts}
\end{figure}

\begin{figure*}[t]
    \centering
    \includegraphics[width=1\linewidth]{graphics/text_similarity.png}
    \caption{Comparison of textual, clinical similarity between reports.}
    \label{fig:similarity}
\end{figure*}

\subsection{Negation}
Negations are prevalent in medical reports, as illustrated in \cref{fig:negngram}, where negated terms dominate the dataset. Unlike general domains, medical reports use diverse negation forms, such as “resolved,” “removed,” or “rule out,” in addition to common terms like “no” or “not.” Understanding negation is critical for accurate model performance, but using negated terms as hard negatives in standard contrastive learning often introduces noise. This is why, even though negations are a serious concern, few studies attempt to tackle this issue.

For example, negating the report “Pneumothorax is present on the right upper lung zone” to “No pneumothorax” would yield a hard negative that overlaps semantically with other normal CXRs or cases without pneumothorax in the same batch, causing confusion. As shown in \cref{fig:entity_value_counts}, using negation as a hard negative will introduce more overlaps as entity counts become smaller in the report. By incorporating dynamic soft labels, we can address this issue, allowing the model to handle clinical semantics effectively without adding noise from negated terms.

\begin{figure}[t]
    \centering
    \includegraphics[width=1\linewidth]{graphics/negation.png}
    \caption{N gram frequent keyword extraction for MIMIC reports. The list is sorted by the top most frequently used phrases.}
    \label{fig:negngram}
\end{figure}

\section{Dataset}
\label{sup:dataset}
\subsection{Dataset Preprocessing}
\label{sec:preprocess}
All CXR images undergo preprocessing through a pipeline that includes monochrome fixation, rotation correction, out-of-distribution (OOD) filtering, and view position selection. The monochrome fixation and rotation correction models were trained on Chexpert dataset using a MobileNetV3 CNN architecture, while view position and OOD detection utilize a DeepMCDD pipeline with a ResNet34 backbone. An example of image post-processing is shown in \cref{fig:ood}. All images are resized to $224 \times 224$ pixels and min-max normalized.

\begin{figure}[t]
    \centering
    \includegraphics[width=1\linewidth]{graphics/ood.png}
    \caption{(a) Data with the lowest OOD score in the MIMIC dataset. (b) Data with the highest OOD score in the MIMIC dataset. The OOD detection model is implemented using the DeepMCDD pipeline.}
    \label{fig:ood}
\end{figure}

\subsection{Dataset Split}
Details of the training, validation, and test splits for our experiments (\cref{ex:main} and \cref{ex:normalthinning}) are provided in \cref{tab:data_summary_vertical}.  We use the same dataset splits as GLORIA~\cite{huang2021gloria} for CheXpert, VinDR, RSNA, and SIIM, while the CXR14 test set follows the split from ProbMed~\cite{probmed}. For MIMIC and OpenI, we exclude lateral and OOD images to ensure data consistency.

\begin{table}[h]
    \centering
    \begin{tabular}{l ccc}
        \toprule
        Dataset & Train & Valid & Test \\
        \midrule
        MIMIC-CXR   & 194,847 & 1,984 & 2,490 \\
        \midrule
        CheXpert   & - & -   & 1000 \\
        VinDR       & -  & - & 3,000 \\
        RSNA        & 18,678  & 4,003 & 4,003 \\
        RSNA-ab       & -   & - & 3,165 \\
        SIIM        & 8,432   & 1,808 & 1,807 \\
        Open-I      & -       & -     & 3,318 \\
        CXR14       & -       & -     & 880 \\
        \bottomrule
    \end{tabular}
    \caption{Data Summary for training and evaluation.}
    \label{tab:data_summary_vertical}
\end{table}

\subsection{CXR-Align}
\label{sec:cxrneg2}
\subsubsection{Counts}
The number of test samples for each dataset in CXR-Align is shown in \cref{table:dataset_count} and the distribution of selected entities is illustrated in \cref{fig:bar}. Entities are randomly selected with weights following the original distribution across test sets. Note that we prioritize cardiomegaly, atelectasis, edema, pleural effusion, pneumothorax, and consolidation, since the generated negations occur more often compared to other entities.

\begin{table}[h!]
\centering
\begin{tabular}{|c|c|c|}
\hline
\textbf{Dataset} & MIMIC & OpenI \\
\hline
\textbf{Count} & 2323 & 953 \\
\hline
\end{tabular}
\caption{Count of datasets used in the \textit{CXR-Align}.}
\label{table:dataset_count}
\end{table}

\begin{figure*}[t]
    \centering
    \includegraphics[width=1\linewidth]{graphics/barplot.png}
    \caption{The number of selected entities in each dataset for CXR-Align.}
    \label{fig:bar}
\end{figure*}

\begin{figure}[t]
    \centering
    \includegraphics[width=1\linewidth]{graphics/example_neg.png}
    \caption{Example of the CXR-Align generation process.}
    \label{fig:exampleneg}
\end{figure}

\subsubsection{Process}
\label{sub:prompt_neg}
The process of CXR-Align generation is shown in \cref{fig:exampleneg}. The removal of findings is a very important step to avoid contradictions or inconsistencies within the report. When mediastinal-related finding is chosen, we add one of the following sentences into the report: 'The cardiomediastinal silhouette is normal.', 'The cardiac silhouette is unremarkable.', 'The heart size is normal.', 'The cardiomediastinal silhouette is within normal limits.', or 'No cardiomegaly.'. If other findings are chosen, we add one of the following templates: "No (finding) is seen.", "No (finding) is observed.", "There is no (finding).", or "No evidence of (finding).". Note that the negated sentence is inserted randomly within the report, either at the beginning, middle, or end. If all the sentences related to the finding were removed, we simply insert the negated statement.

\subsubsection{Prompts}
Below is the prompt for each step in LLM text preprocessing as in \cref{fig:cxrneg}.
\paragraph{Splitting}
We use the prompt from MAIRA2~\cite{maira2} for splitting reports so that each sentence represent and describe only one entity.
\paragraph{Removing Prior Reference}
"You are an expert chest X-ray (CXR) radiologist familiar with radiologic reports. Your task is to rewrite the given radiology reports by removing all references to prior reports or comparisons, while preserving the original structure as much as possible.
Input: A radiology report for a chest X-ray (CXR).
Output: A revised CXR report focusing solely on current medical findings, excluding references to prior reports, comparisons, and irrelevant details.
Guidelines:
Remove Comparisons: Eliminate any terms or phrases that suggest a comparison, such as "compared to," "in comparison with," "change", "cleared", "constant", "decrease", "elevate", "expand", "improve", "decrease", "increase", "persistent", "reduce", "remove", "resolve", "stable", "worse", "new", etc.
Focus on Current Findings: Ensure the report only describes the current state of the patient's lungs and related structures.
Preserve Medical Context: Maintain the original medical terminology and descriptions of abnormalities.
Retain Negations: Keep any negative statements about the absence of abnormalities.

Example 1:
Original: The left apex has not been included on this radiograph. The ET tube terminates 3.9 cm above the carina. The NG tube terminates in the stomach. Surgical clips and a faint metallic coil project over the chest. A left PICC terminates in the mid SVC. EKG leads overlie the chest wall. The lung volumes are low. There are persistent bilateral mid and lower zone hazy opacities. There are persistent bilateral hilar and perihilar linear opacities. No significant interval change is observed in the lung opacities. Bilateral pleural effusions are present. The right pleural effusion is greater than the left. No pneumothorax is observed on the right. No cardiomegaly is present. No interval change is observed in the mediastinal silhouette. No significant interval change is observed in the bony thorax.  
Revised: The left apex has not been included on this radiograph. The ET tube terminates 3.9 cm above the carina. The NG tube terminates in the stomach. Surgical clips and a faint metallic coil project over the chest. A left PICC terminates in the mid SVC. EKG leads overlie the chest wall. The lung volumes are low. There are persistent bilateral mid and lower zone hazy opacities. There are bilateral hilar and perihilar linear opacities. Bilateral pleural effusions are present. The right pleural effusion is greater than the left. No pneumothorax is observed on the right. No cardiomegaly is present. "

\paragraph{Omitting selected entity}
"Task: Given a specific finding or disease and a chest X-ray report, remove the sentences relevant to that finding or disease.

Context:

Lung lesion: Refers to nodule or mass.
Pleural other: Refers to pleural thickening.

Example:

Finding: Lung Lesion
Report: No pneumothorax is observed. No pleural effusion is observed. No evidence of hemorrhage is observed in the lung or mediastinum. Emphysema is severe. The heart size is normal. A complex of nodule and large bullae is present in the axillary region of the right upper lobe. 
Expected Output: No pneumothorax is observed. No pleural effusion is observed. No evidence of hemorrhage is observed in the lung or mediastinum. Emphysema is severe. The heart size is normal.

Finding: Cardiomegaly
Report: The feeding tube, with the wire stylet in place, is in the mid stomach. Heterogeneous pulmonary opacification is most pronounced in the left mid and lower lung. Heterogeneous pulmonary opacification is also present on the right, sparing only the upper lobe. The heart is mildly enlarged.
Expected Output: The feeding tube, with the wire stylet in place, is in the mid stomach. Heterogeneous pulmonary opacification is most pronounced in the left mid and lower lung. Heterogeneous pulmonary opacification is also present on the right, sparing only the upper lobe."

\subsection{Normal Case Detection} As described in \cref{ex:normalthinning}, we augmented the MIMIC dataset by adding 130,000 normal CXR images from a single tertiary hospital, each labeled with the report “No active lung lesion.” This augmentation results in an imbalanced dataset with 176,726 normal CXRs and 148,121 abnormal CXRs in the training set. For the reports which is used for the test set of this task, we included 2,999 abnormal reports sampled from the MIMIC test set with one normal report "No active lung lesion.". Data counts for the normal case detection experiment are provided in \cref{tab:data_summary_normalthinning}.
\begin{table}[h]
    \centering
    \begin{tabular}{l ccc}
        \toprule
        Dataset & Train & Valid & Test \\
        \midrule
        MIMIC-CXR   & 194,847 & - & - \\
        Private     & 130,000 & - & 1,026 \\
        \midrule
        Open-I      & -       & -     & 1,289 \\
        \bottomrule
    \end{tabular}
    \caption{Data counts for normal case detection experiment.}
    \label{tab:data_summary_normalthinning}
\end{table}

\subsection{Dataset Approvals and Ethics}

All procedures involving the MIMIC dataset, including large language model (LLM)-assisted report preprocessing and the construction of CXR-Align, were conducted in full compliance with PhysioNet’s guidelines for responsible LLM usage (\url{https://physionet.org/news/post/gpt-responsible-use}). Use of the private dataset was approved by the Institutional Review Board (IRB), with all researchers formally registered and authorized for data access. Due to licensing restrictions, only the MIMIC-based version of CXR-Align will be shared via PhysioNet, and access will be limited to credentialed users.

\section{Model}
\label{sec:model_info}
This section details the model implementation, augmentations, details with clinical information and hyperparameters.

\subsection{Implementation Details} The model is trained using the AdamW optimizer with a cosine learning rate schedule and linear warm-up. The learning rate is set to $4 \times 10^{-6}$, with a batch size of 64 over 10 epochs on a single A6000 GPU. For fine-tuning experiments, we set the learning rate to $1 \times 10^{-4}$, with a batch size of 128. We train for 200 epochs when fine-tuning with 10\% of the data, and for 20 epochs when fine-tuning with 100\% of the data, all on a single A6000 GPU. Each graph node's word is embedded using ClinicalBERT, and a one-hot code for class 'ANAT-DP', 'OBS-DP', 'OBS-DA', and 'OBS-U' is concatenated. The Graph Convolutional Neural Network (GCNN) for graph embeddings consists of two GCN conv layers with an input dimension of 772, a hidden dimension of 256, and an output dimension of 512 which is same with the other modalities.  The max token length is set to 300.

\subsection{Augmentations} For image augmentation, we apply Contrast Limited Adaptive Histogram Equalization (CLAHE) with a clip limit of 4, random resized cropping, and rotations of up to 10 degrees. Text augmentation consists of sentence shuffling only.

\subsection{Clinical Information} For the clinical information, we use CheXbert to extract the presence of entities. We additionally add one more label, where the value is 1 if all other labels are 0, and 0 otherwise. This accounts for cases where no findings are present, including entities that CheXbert may not cover. The entities are: [
        "Cardiomegaly", "Lung Opacity", "Atelectasis", "Lung Lesion", 
        "Pleural Effusion", "Fracture", "Support Devices", 
        "Enlarged Cardiomediastinum", "Pleural Other", 
        "Consolidation", "Edema", "Pneumothorax", "Pneumonia", "No Findings"].

\subsection{Hyperparameters}
\label{sub:hyper}
The temperature \(\tau\) is set to 0.1, and similarity thresholds for textual \(\tau_t\), clinical  \(\tau_c\), graph  \(\tau_g\) set at  0.9, 0.8, and 0.7, respectively. The weights for text \(w_T\), clinical \(w_C\), graph \(w_G\) weights in \cref{eq:final} are all set to 0.167.

\section{Evaluation Settings}
\subsection{zero-shot prompt}
Zero-shot prompt used for \cref{ex:main} is shown in \cref{table:findings}. For CheXpert multi-class classification, we follow the prompt used in CXR-CLIP. For adversarial prediction, we used the same prompts as in the "Others" category.
\begin{table}[h!]
\footnotesize
\centering
\begin{tabular}{|l|l|l|}
\hline
            & \textbf{Positive}                             & \textbf{Negative}                             \\ \hline
\textbf{RSNA}   & Findings suggesting pneumonia.               & No evidence of pneumonia.                     \\ \hline
\textbf{SIIM}   & There is pneumothorax                       & There is no pneumothorax                      \\ \hline
\textbf{Others} & There is \{findings\}                       & There is no \{findings\}                      \\ \hline
\end{tabular}
\caption{Positive and negative prompts for zero-shot evaluation.}
\label{table:findings}
\end{table}

\subsection{Report retrieval}
For report retrieval, we use the CheXbert F1 score rather than the standard BERTScore to evaluate how the retrieved or generated report clinically reflects the original report. The Macro F1 score is used since the Micro F1 score does not reflect the imbalance of the dataset.  Furthermore, rather than focusing on top-\(k\) retrieval performance, we emphasized clinical metrics because the test set contains reports with similar clinical semantics, which could bias the performance evaluation if based solely on top-\(k\) retrieval metrics.

\section{Additional Experiment}
\label{sec:sup_ex}

In this section, we provide a detailed discussion of our experiments. A notable finding from \cref{ex:main} is that our model's performance improves as we incorporate each similarity measure and hard negatives. Surprisingly, our baseline CLIP model's finetuned performance is comparable to or surpasses most of the SOTA CLIP models, implying that preprocessing steps like splitting reports and omitting prior references enhance the discriminability of CLIP models. Furthermore, adding similarity measures narrowed the gap between the RSNA and RSNA-\(ab\) results, indicating that our method helps the model to discriminate and correctly identify entities within abnormalities. In the following subsections, we provide a more detailed analysis of our benchmark \textit{CXR-Align}, adversarial prediction, normal case detection, and report retrieval.

\subsection{Detailed analysis on CXR-Align}
\cref{fig:mimicneg} and \cref{fig:openineg} provide a detailed sub-analysis for the \textit{CXR-Align} benchmark on the MIMIC, and OpenI datasets, respectively. We analyze the following aspects:
\begin{enumerate}[leftmargin=*] \item \textbf{Entity Type}: For all datasets, negated entities related to 'pneumothorax', 'effusion', 'consolidation', 'enlarged cardiomediastinum', and 'pneumonia' performed below average, while the model best discriminated 'pleural other', 'support devices', and 'fracture'. This may be due to the prompts used to negate the latter entities being less frequent in the training set compared to the former. \item \textbf{Location}: The insertion location of the negation did not significantly affect performance, as accuracy was similar across all positions. \item \textbf{Mediastinal Prompt}: For prompts regarding mediastinal findings, Prompt 2 ('The heart size is normal') consistently resulted in below-average accuracy when inserted as a negated statement across all datasets. \item \textbf{Other Prompts}: For prompts related to lung entities, Prompt 2 ("There is no {finding}") performed the worst, falling below average. However, all prompts exhibited similar accuracy overall. \end{enumerate}

We hypothesize that the frequency of negated terms for each entity or prompt affects the model's performance and its comprehension of negations.

\subsection{Detailed analysis on Adversarial Prediction}
In this section, we perform a detailed analysis of adversarial prediction. We investigate how different models behave when subjected to this task compared to our model. As described in \cref{ex:adverserial}, this complex zero-shot task requires the model to determine whether one entity is present and another is absent. We conducted a total of 1,915 adversarial classification tasks. As shown in \cref{tab:adv_comparison} most SOTA models tend to predict an entity as positive when given an abnormal CXR, indicating that they do not effectively discern which entities are present or absent. This raises concerns about the zero-shot classification task discussed in \cref{ex:main} suggesting that models may focus on the overall abnormality of the CXR rather than understanding the full context and associating positivity with specific entities. While CXR-CLIP mitigated this issue to some extent, our model demonstrated better clinical understanding regarding the presence and absence of clinical findings.

\begin{table}[h]
    \centering
    \begin{tabular}{l c c c c}
        \toprule
        GT & \multicolumn{2}{c}{Present} & \multicolumn{2}{c}{Absent} \\
        \cmidrule(lr){2-3} \cmidrule(lr){4-5}
        Model & Positive & Negative & Positive & Negative \\
        \midrule
        GLORIA & 1671 & 244 & 1696 & 219 \\
        BioViL & 1539 & 376 & 1281 & 634 \\
        BioViL-T & 1625 & 290 & 1455 & 460 \\
        CXR-CLIP & 754 & 1161 & 341 & 1574 \\
        \midrule
        OURS & 720 & 1195 & 195 & 1720 \\
        \bottomrule
    \end{tabular}
    \caption{Positive/negative prediction counts in the adversarial prediction task for each model.}
    \label{tab:adv_comparison}
\end{table}

\subsection{Detailed Analysis on Normal Case Detection}
We conducted a detailed analysis of normal case detection, where the model must retrieve one normal report from 2,999 abnormal reports. As shown in \cref{tab:normal_skew},  training with long-tailed data containing more than 50\% normal CXR reports enables the model to effectively retrieve the normal report among all other abnormal reports. For the model trained only on the MIMIC dataset, the rank of the normal report was 68th. When using our internal test set as in \cref{tab:data_summary_normalthinning}, the model successfully retrieved the normal report with 99.7\% accuracy. This suggests that further training with internal data containing normal CXRs can achieve higher performance for internal tasks, allowing hospitals to build their own specialized models.

\begin{table}[h!]
\centering
 % Adjust row spacing for readability
\begin{tabular}{|p{0.8\columnwidth}|r|}
\hline
\multicolumn{2}{|c|}{\textbf{OURS\(_{mimic}\)}} \\
\hline
There is a right lower lobe airspace consolidation. The lungs are otherwise clear. The hilar and cardiomediastinal contours are normal. There is no pneumothorax. There is no pleural effusion. Pulmonary vascularity is normal.  & 12 \\
\hline
A small residual area of linear atelectasis is present in the retrocardiac area. No pneumothorax is observed. No pleural effusion is observed. The heart size is normal. The hilar contours are normal. The mediastinal contours are normal. The visualized osseous structures are unremarkable. & 12 \\
\hline
The heart is normal in size. The mediastinal and hilar contours appear within normal limits. There is an inferolateral consolidation in the right upper lobe, consistent with pneumonia. The lungs appear clear elsewhere. No pleural effusions are present. No pneumothorax is present. The osseous structures are unremarkable. & 11 \\
\hline
\multicolumn{2}{|c|}{\textbf{OURS\(_{mimic+private}\)}} \\
\hline
No active lung lesion. & 1105 \\
\hline
No focal consolidation is seen. No pleural effusion is seen. No pneumothorax is seen. No pulmonary edema is seen. Minimal bronchial wall thickening is present. The heart size is normal. Mediastinal contours are normal. No bony abnormality is detected. & 48 \\
\hline
No lung consolidation. The left lower lung atelectatic band has resolved. Mediastinal and cardiac contours are normal. No pneumothorax. No pleural effusion. & 14 \\
\hline
\end{tabular}
\caption{Most frequent reports and their counts retrieved from the normal case detection task for the OpenI test images. The upper table shows results for our model trained only on MIMIC, while the lower table shows results for our model trained on MIMIC and private data.}
\label{tab:normal_skew}
\end{table}

\subsection{Report Retrieval}
We provide examples of report retrieval performance in \cref{fig:retrieved}. Compared to other SOTA models and the baseline model, our model successfully retrieves reports that share similar semantics with the original report, even if they are not identical. Notably, in the third example, our model linked the textual semantics of "There is infrahilar interstitial prominence which may represent bronchovascular crowding lung" to the original report's "The lungs are hypoinflated," demonstrating high correlation.

\section*{Acknowledgments}  We would like to thank H.Y. Cho, I.H. Baek and Y.G. Kim for their valuable advice on this paper. This study was supported by the National Research Foundation of Korea (NRF) grants funded by the Ministry of Science and ICT (MSIT) (Grant No. RS-2024-00354666).

\section*{Comment on Manuscript Version}
This is the author-accepted manuscript of our paper accepted to the IEEE/CVF Conference on Computer Vision and Pattern Recognition (CVPR) 2025. This version includes an expanded ethics and data user agreement section, which was not part of the original submission to CVPR. The added section provides further transparency and compliance with data usage policies.

\begin{figure*}[t]
    \centering
    \includegraphics[width=1\linewidth]{graphics/retrieval_image.png}
    \caption{Examples of retrieved reports. Blue text represents important entities that should be included in the report. Red text indicates hallucinations or falsely interpreted entities. Purple represents clinically similar entities.}
    \label{fig:retrieved}
\end{figure*}

\begin{figure*}[t]
    \centering
    \includegraphics[width=0.8\textwidth]{graphics/mimic-acc.png}
    \caption{Detailed sub-analysis for CXR-Align on MIMIC dataset. (A) Task accuracy for entities that were either negated or removed. (B) Performance based on the location where the negated sentence was inserted. (C) Accuracy corresponding to the prompt used when the selected entity was related to mediastinal findings. (D) Performance corresponding to the prompt used when the selected entity was related to lung findings. For (C) and (D), refer to \cref{sub:prompt_neg}}
    \label{fig:mimicneg}
\end{figure*}

\begin{figure*}[t]
    \centering
    \includegraphics[width=0.8\textwidth]{graphics/openi-acc.png}
    \caption{Detailed sub-analysis for CXR-Align on OPENI dataset. (A) Task accuracy for entities that were either negated or removed. (B) Performance based on the location where the negated sentence was inserted. (C) Accuracy corresponding to the prompt used when the selected entity was related to mediastinal findings. (D) Performance corresponding to the prompt used when the selected entity was related to lung findings. For (C) and (D), refer to \cref{sub:prompt_neg}}
    \label{fig:openineg}
\end{figure*}
